# Supplementary material for: VISCR: Intuitive & Conflict-free Automation for Securing the Dynamic Consumer IoT Infrastructures
Source: arXiv:1907.13288 source file (2019-07-31)
Supplement: Supplementary file 1 [file appendix_vise.tex]

\begin{figure}[h!]
\vspace{-15pt}
\includegraphics{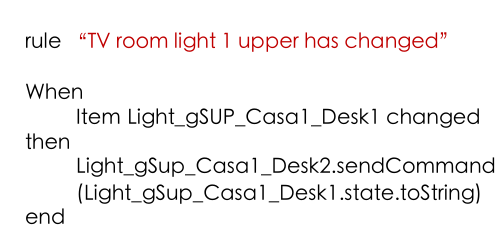}
\vspace{-15pt}
\caption{Sample OpenHAB program snippet.}\label{figure:openhab_iot_rule}
% \vspace{-15pt}
\end{figure}

\begin{figure}[h!]
\vspace{-15pt}
\begin{center}
\begin{subfigure}[b]{0.23\textwidth}
\includegraphics{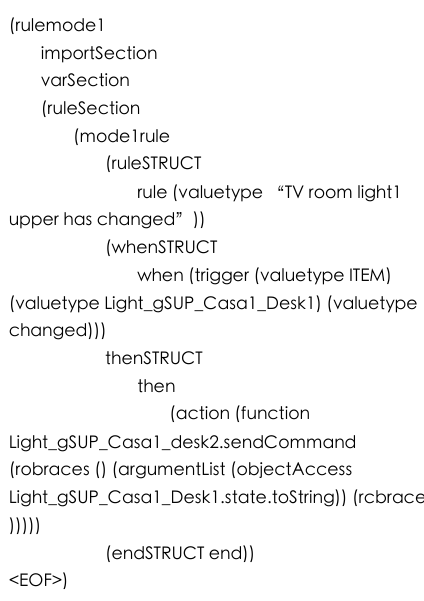}
\caption{Abstracted LISP Representation (ALR) of Policy.}\label{figure:alr}
\end{subfigure}\hfill
\begin{subfigure}[b]{0.23\textwidth}
\includegraphics{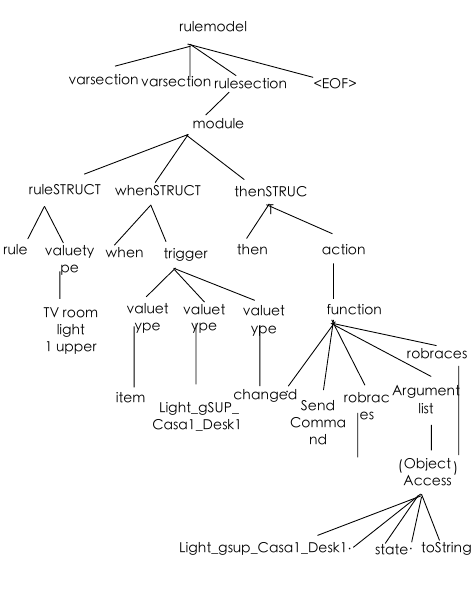}
\caption{Abstracted Tree Representation (ATR) of Policy.}\label{figure:atr}
\end{subfigure}
% \vspace{-5pt}
\end{center}
% \vspace{-15pt}
\caption{\small Equivalent Intermediate Abstracted LISP and Tree representation of OpenHAB policy shown in Figure \ref{figure:openhab_iot_rule}.}\label{figure:vi_alr_alg_translation}
\end{figure}
